# Supplementary material for: Towards Optimal Regret in Adversarial Linear MDPs with Bandit Feedback
Source: arXiv:2310.11550 source file (2023-10-17)
Supplement: Supplementary file 1 [file appendix-proof-sketch-efficient.tex]

\section{Proof Sketch for the Efficient Algorithm}

To control the magnitude and variance of the bonus, our efficient algorithm relies on having an initial pure exploration phase for the first $K_0$ episodes to estimate the transition of the MDP to a certain degree. The method is inspired by \cite{sherman2023rate} and built upon the reward-free exploration algorithm developed by \cite{wagenmaker2022reward}. The related techniques are well-documented in \cite{wagenmaker2022reward, sherman2023rate}, which we just use in a standard way. Therefore, we only summarize the guarantee in the following lemma, and leave all the details in \pref{app: pure exploration}.

\begin{lemma}
\label{lem:goodevent_rfw}
	For linear MDPs, with inputs $\delta\in(0,1)$, $\rho>0$, $\epsilon_{\rm cov}>0$, \pref{alg:reward_free} will terminate in $T=\widetilde{\Theta}\left( \frac{dH/\rho^2 + d^4 H^4}{\epsilon_{\rm cov}} \polylog\left(\frac{1}{\delta}, \frac{1}{\rho}, \frac{1}{\epsilon_{\rm cov}}, d, H\right)\right)$ episodes, and output 
    $H$ datasets $\{\calD_{h}\}_{h=1}^H$ where $\calD_h\subset \calS_h\times \calA\times \calS_{h+1}$ such that with probability $\geq 1-\delta$, 
	\begin{align*}
		\forall h, \forall \pi, \quad 
  \sum_{s\in\calS_h} \mu^\pi(s) \ind\{s\notin \calZ_h\} \leq \epsilon_{\rm cov},
		 \text{\ \ where\ \ } 
		 \calZ_h \triangleq \left\{s\in \calS_h:~~ \forall a\in\calA,\ \  \norm{\phi(s, a)}_{\Lambda_{h}^{-1}}\leq \rho\right\} 
	\end{align*} 
with
    $
         \Lambda_h \triangleq I + \sum_{(s,a,s')\in \calD_h} \phi(s,a)\phi(s,a)^\top.  
   $
   % If the MDP is a $\zeta$-misspecified linear MDP with $\zeta\leq \order\left(\frac{1}{\poly(d,H)T^3}\right)$, the same guarantee holds. 
\end{lemma}

%Note that although \cite{luo2021policy} and \cite{dai2023refined} also set up an initial exploration phase, their purpose is different from ours. Namely, they utilize the policy cover idea proposed in \cite{agarwal2020pc} and \cite{zanette2021cautiously} to learn a mixture policy $\pi_{\rm cov}$ and its corresponding covariance matrix $\hatSigma_{h}^{\rm cov}$ such that $\|\phi(s,a)\|_{\left(\hatSigma_{h}^{\rm cov}\right)^{-1}}$ is small for most states $s$ with any action $a$. With this guarantee, by executing $\pi_{\rm cov}$ in certain episodes and only adding a bonus for the state that $\|\phi(s,a)\|_{\left(\hatSigma_{h}^{\rm cov}\right)^{-1}}$ is small, the magnitude of bonus could be controlled. Our bonus design follows the idea in \cite{sherman2023improved}, which gets rid of the policy cover phase but introduces an additional optimistic exploration term $\|\phi(s,a)\|_{\Lambda_h^{-1}}^2$ where $\Lambda_{h} = I + \sum_{(s,a) \in D_h} \phi(s, a)^\top \phi(s, a)$ for a given dataset $D_h = \{(s_{i,h}, a_{i,h})\}_{i=1}^{|D_h|}$. In order to control $\|\phi(s,a)\|_{\Lambda_h^{-1}}^2$, we conduct the initial exploration phase to collect $D_h$ and use \pref{lem:goodevent_rfw}  to ensure it is small for almost all states.

One of the main purposes of our initial exploration phase is to control the magnitude of the bonus calculated by \pref{alg: dilated bonus}. 
Specifically, in the constrained linear regression (Line 5) of \pref{alg: dilated bonus}, the $\widehat{w}_{k,h}$ is the estimation of 
\begin{align}
    w_{k,h} = \sum_{s' \in \calS_{h+1}}\psi(s')y(s')\ind\{s' \in \calZ_{h+1}\}
\label{eqn:true w}
\end{align}
By setting $\epsilon_{\rm cov} = K^{-\frac{1}{4}}$ and $\rho = K^{-\frac{1}{4}}$ in \pref{alg:reward_free}, from \pref{lem:goodevent_rfw}, the exploration phase will terminate in $\otil\left(K^{\frac{3}{4}}\right)$ rounds and for any $s \in \calZ_h$, $\|\phi(s,a)\|_{\Lambda_{k,h}^{-1}}^2 \le K^{-\frac{1}{2}}$. This implies that  $\|w_{k,h}\|_2 \le B^{\max} = H\sqrt{d}\left(\frac{\beta}{\gamma} + \frac{\alpha}{\sqrt{K}}\right) = \order\left(H\sqrt{d}K^{\frac{1}{4}}\right)$.
Since the optimization for $\widehat{w}_{k,h}$ searches in the region of $w_{k,h}$, we could derive the following lemma.
\begin{lemma}
For any $s,a,k,h$, if $\beta' = \otil\left(B^{\max}\right)$,  with high probability, given $\alpha = \order\left(K^{\frac{3}{4}}\right)$ we have
\begin{align*}
    \left|\phi(s,a)^\top\left(\widehat{w}_{k,h} - w_{k,h}\right)\right| \le \beta' \|\phi(s,a)\|_{\Lambda_{k,h}^{-1}} \le \otil\left(K^{-\frac{1}{4}}\right) + \alpha\|\phi(s,a)\|^2_{\Lambda_{k,h}^{-1}}
\end{align*}
\label{lem: difference bound main}
\end{lemma}
The initial exploration phase ensures a smaller $B^{\max}$ and thus a smaller $\frac{(\beta')^2}{4\alpha}$. This serves as a key point for improving regret. When analyzing the regret, several bounds only hold for state $s \in \calZ_h$, this motivates us to divide trajectories based on their states. For any trajectory $t = \{(s_h, a_h)\}_{h=1}^H$ generated by any policy, if $s_h \in \calZ_h$ for any $h \in [H]$, then we say $t$ is a \textit{good trajectory}. From \pref{lem:goodevent_rfw} and union bound, with probability $1 - HK^{-\frac{1}{4}}$, $t$ is a \textit{good trajectory} no matter which policy it comes from. 
To better conduct analysis based on trajectories, we define $T_{h}^{\pi}$ be the distribution of trajectory $\{(s_i, a_i)\}_{i=1}^h$ for the first $h$ steps generated by  policy $\pi$ and transition $\mathbb{P}$, we define $\E_h^{\pi} \left[\cdot\right] = \E_{\tau_{h-1} = \{(s_i, a_i)\}_{i=1}^{h-1} \sim T_{h-1}^{\pi}}\E_{s_h \sim \mathbb{P}(s_h \mid s_{h-1}, a_{h-1})}\left[\cdot\right]$. For any $h$ and random variable $X$ that only depends on $s_h$, by the markov property, we have $\E_{s_h \sim \mu_h^{\pi}}\left[X\right] = \E_h^{\pi}\left[X\right]$. For any trajectory with state sequence $\{s_i\}_{i=1}^h$ with length $h$, define event $\calE_h$ as the event that $\forall h' \le h, s_{h'} \in \calZ_{h'}$. 
In the following analysis, we will mainly consider policy $\pi_k$ for each episode $k$ and the optimal policy $\pi^\star$. For notation simplicity, we set $\E_{h}^{\pi_k}\left[\cdot\right] = \E_{h}^k\left[\cdot\right]$ and  $\E_{h}^{\pi^\star}\left[\cdot\right] = \E_{h}^\star\left[\cdot\right]$.

By performance difference lemma \cite{kakade2002approximately}, we have
\begin{align}
    \E\left[\Reg\right] &= \E\left[\sum_{k=1}^K \sum_{h=1}^H \E_{s \sim \mu_h^\star}
			\left[ \left\langle Q_{k,h}(s, \cdot), 
				\pi_{k}(\cdot|s) - \pi^\star(\cdot|s) \right\rangle \right]\right] = \E\left[\sum_{k=1}^K \sum_{h=1}^H \E_h^\star
			\left[ \left\langle Q_{k,h}(s, \cdot), 
				\pi_k(\cdot|s) - \pi^\star(\cdot|s) \right\rangle \right]\right] \nonumber
		\\&=\E\left[\sum_{k=1}^K \sum_{h=1}^H \E_h^\star
			\left[ \left\langle Q_{k,h}(s, \cdot), 
				\pi_k(\cdot|s) - \pi^\star(\cdot|s) \right\rangle \ind\{\calE_h\}\right] 
    + \sum_{k=1}^K \sum_{h=1}^H \E_h^\star
			\left[ \left\langle Q_{k,h}(s, \cdot), 
				\pi_k(\cdot|s) - \pi^\star(\cdot|s) \right\rangle\ind\{\overline{\calE_h}\}\right]\right]  \nonumber
        \\&\le \underbrace{\E\left[\sum_{k=1}^K \sum_{h=1}^H \E_h^\star
			\left[ \left\langle Q_{k,h}(s, \cdot), 
				\pi_k(\cdot|s) - \pi^\star(\cdot|s) \right\rangle \ind\{\calE_h\}\right]\right]}_{\textbf{REG-TERM}} + H^3K^{\frac{3}{4}} \tag{$\mathrm{Pr}\left(\overline{\calE_h}\right) \le HK^{-\frac{1}{4}}$}
\label{eqn:regret decomposition}
\end{align}
Thus, the remaining task is to bound the cumulative regret $\textbf{REG-TERM}$ for good trajectories. To do so, in our bonus design, we utilize the technique of ``dilated bonus'' which is first proposed in \cite{luo2021policy} and is also used in \cite{dai2023refined}. The motivation of the dilated bonus is that the regret usually contains $\sum_{k=1}^K\sum_{h=1}^H\E_{s \sim \mu_h^\star}\E_{a \sim \pi^\star(\cdot|s)}\left[b_{k,h}(s,a)\right]$ for some non-negative $b_{k,h}(s,a)$, which could be potentially large. On the other hand, $\sum_{k=1}^K\sum_{h=1}^H\E_{s \sim \mu_h^k}\E_{a \sim \pi_k(\cdot|s)}\left[b_{k,h}(s,a)\right]$ is usually well-bounded. The ``dilated bonus'' serves as a technique to design bonus in order to convert the measure from $\pi^\star$ to $\pi_k$ to ensure the regret bound. \pref{lem:dilated bonus guarantee} summarizes this theorem where we do a slight change of expectation measure. The proof can be found in \pref{app:efficient}.

\begin{lemma}[Lemma 3.1 in \cite{luo2021policy}]
If $b_{k,h}(s,a)$ be non-negative for any $k,h,s \in \calS_h,a$ and we have
\begin{equation}
B_{k,h}(s,a) \ge b_{k,h}(s,a) + \left(1 + \frac{1}{H}\right)\E_{s' \sim \mathbb{P}(\cdot|s,a)}\E_{a' \sim \pi_k(\cdot|s')}\left[B_{k,h}(s', a')\ind\{s' \in \calZ_{h+1}\}\right] - f(K)
\label{eqn:B condition}
\end{equation}
and the following holds
\begin{align}
    &\E\left[\sum_{k=1}^K\sum_{h=1}^H\E_h^\star\left[\left\langle Q_{k,h}(s,\cdot) - B_{k,h}(s,a), \pi_k(\cdot|s) - \pi^\star(\cdot|s)\right\rangle\ind\{\calE_h\}\right] \right] \nonumber
    \\&\le g(K) + \E\left[\sum_{k=1}^K\sum_{h=1}^H\E_h^\star\E_{a \sim \pi^\star(\cdot|s)}\left[b_{k,h}(s,a)\ind\{\calE_h\}\right]\right]  + \frac{1}{H}\E\left[\sum_{k=1}^K\sum_{h=1}^H\E_h^\star\E_{a \sim \pi_k}\left[B_{k,h}(s,a)\ind\{\calE_h\}\right]\right]
\label{eqn:regret condition}
\end{align}
where $f(K), g(K)$ could be any function that only depends on $K$. Then, we have
\begin{align*}
    \textbf{REG-TERM} \le g(K) + HKf(K) + \left(1+\frac{1}{H}\right)\E\left[\sum_{k=1}^K\E_{a \sim \pi_k(\cdot|s_1)}\left[B_{k,1}(s_1,a)\ind\{\calE_1\}\right] \right]
\end{align*}
\label{lem:dilated bonus guarantee}
\end{lemma}
Recall the definition of $w_{k,h}$ in \pref{eqn:true w}, from the definition of linear MDP, for all $k,h,s,a$, we have 
\begin{align}
&\phi(s,a)^\top w_{k,h} \nonumber 
\\&= \E_{s' \sim \mathbb{P}(\cdot|s,a)}\left[y(s')\ind\{s' \in \calZ_{h+1}\}\right] \nonumber
\\&=  \E_{s' \sim \mathbb{P}(\cdot|s,a)}\E_{a' \sim \pi_k(\cdot| s)}\left[\left(\beta\|\phi(s',a')\|^2_{\hatSigma_{k, h+1}^{-1}} + 2\alpha \|\phi(s',a')\|^2_{\Lambda_{k, h+1}^{-1}} + \left(1+\frac{1}{H}\right)\widehat{B}_{k,h+1}^+(s',a')\right)\ind\{s' \in \calZ_{h+1}\}\right] 
% \left(1+\frac{1}{H}\right)\E_{s \sim \mathbb{P}(\cdot|s,a)}\E_{a \sim \pi_k(\cdot|s)}\left[\widehat{B}_{k,h+1}^+(s,a)\right]  
% \\&\ge \E_{s' \sim \mathbb{P}(\cdot|s,a)}\E_{a' \sim \pi_k(\cdot| s)}\left[\left(\beta\|\phi(s',a')\|^2_{\hatSigma_{k, h+1}^{-1}} + 2\alpha \|\phi(s',a')\|^2_{\Lambda_{k, h+1}^{-1}}\right)\ind\{s' \in \calZ_{h+1}\} + \left(1+\frac{1}{H}\right)\widehat{B}_{k,h+1}^+(s',a')\right] 
\label{eqn: lower bound E}
\end{align}

Let $B_{k,h} = \beta\|\phi(s,a)\|_{\hatSigma^{-1}_{k,h}}^2 + \phi(s, a)^\top w_{k,h} +   \alpha \|\phi(s,a)\|_{\Lambda_{k, h}^{-1}}^2$ which using the true feature $w_{k,h}$ instead of  $\widehat{w}_{k,h}$ in $\widehat{B}_{k,h}$. In order to convert $\widehat{B}_{k,h}^+(s, a)$ to $B_{k,h}(s,a)$, we introduce \pref{lem: B main bias} to bound their difference which directly comes from \pref{lem: difference bound main}.
\begin{lemma}
For any $k,h,s,a$,  with high probability, we have
\begin{align*}
\left|\widehat{B}_{k,h}^+(s, a) - B_{k,h}(s, a) \right| \le \left|\widehat{B}_{k,h}(s, a) - B_{k,h}(s, a) \right| \le \otil\left(K^{-\frac{1}{2}}\right)  + \alpha\|\phi(s,a)\|_{(\Lambda_h^k)^{-1}}^2    
\end{align*}
\label{lem: B main bias}
\end{lemma}
Combining \pref{eqn: lower bound E} and \pref{lem: B main bias}, we have 

\begin{align*}
B_{k,h}(s, a) &\ge \left(1+\frac{1}{H}\right) \E_{s' \sim \mathbb{P}(\cdot|s,a)}\E_{a' \sim \pi_k(\cdot|s')}\left[B_{k,h+1}(s',a') \ind\{s' \in \calZ_{h+1}\}\right]+ \beta\|\phi(s,a)\|_{\hatSigma^{-1}_{k,h}}^2 + \alpha \|\phi(s,a)\|_{\Lambda_{k, h}^{-1}}^2 
\\&\qquad + \E_{s' \sim \mathbb{P}(\cdot|s,a)}\E_{a' \sim \pi_k(\cdot|s')}\left[
\left(\beta\|\phi(s',a')\|^2_{\hatSigma_{k, h+1}^{-1}} + \alpha\|\phi(s',a')\|^2_{\Lambda_{k, h+1}^{-1}}\right)\ind\{s' \in \calZ_{h+1}\}\right] - \otil\left(K^{-\frac{1}{2}}\right)
\end{align*}

Define 
\begin{align}
 &b_{k,h}(s,a) \nonumber
 \\&= \beta\|\phi(s,a)\|_{\hatSigma^{-1}_{k,h}}^2 + \alpha \|\phi(s,a)\|_{\Lambda_{k, h}^{-1}}^2 +  \E_{s' \sim \mathbb{P}(\cdot|s,a)}\E_{a' \sim \pi_k(\cdot|s')}\left[
\left(\beta\|\phi(s',a')\|^2_{\hatSigma_{k, h+1}^{-1}} + \alpha\|\phi(s',a')\|^2_{\Lambda_{k, h+1}^{-1}}\right)\ind\{s' \in \calZ_{h+1}\}\right] 
\label{eqn: b define}
\end{align}
Since $b_{k,h}(s,a) \ge 0$ are non-negative for all $s,a$, bonus $B_{k,h}$ satisfies the condition in \pref{lem:dilated bonus bound}. Furthermore, for any random variable $X$, since
\begin{equation}
\E_h^\star\E_{a \sim \pi^\star(\cdot|s)}\E_{s' \sim \mathbb{P}(\cdot|s,a)}\left[X \ind\{\calE_h\}\ind\{s' \in \calZ_{h+1}\}\right] = \E_{h+1}^\star\left[X\ind\{\calE_{h+1}\}\right]
\label{eqn:expectation eq}
\end{equation}
We have
\begin{align*}
&\sum_{k=1}^K\sum_{h=1}^H\E_h^\star\E_{a \sim \pi^\star(\cdot|s)}\left[b_{k,h}(s,a)\ind\{\calE_h\}\right] 
\\&= \sum_{k=1}^K\sum_{h=1}^H\E_h^\star\E_{a \sim \pi^\star(\cdot|s)}\left[\left(\beta\|\phi(s,a)\|_{\hatSigma^{-1}_{k,h}}^2 + \alpha \|\phi(s,a)\|_{\Lambda_{k, h}^{-1}}^2\right)\ind\{\calE_h\}\right]
\\&\quad+   \sum_{k=1}^K\sum_{h=2}^H\E_h^\star\E_{a \sim \pi_k(\cdot|s)}\left[
\left(\beta\|\phi(s,a)\|^2_{\hatSigma_{k, h+1}^{-1}} + \alpha\|\phi(s,a)\|^2_{\Lambda_{k, h+1}^{-1}}\right)\ind\{\calE_h\}\right] 
\end{align*}
Note that the last term only takes summation for $h=2, \cdots, H$ because \pref{eqn:expectation eq} considers the next state of $h$. Moreover, it is standard to show $\sum_{k=1}^K\E_{a \sim \pi_k(\cdot|s_1)}\left[B_{k,1}(s_1,a)\ind\{\calE_1\}\right]  \le \otil\left(K^{\frac{3}{4}}\right)$. Thus, in order to use \pref{lem:dilated bonus bound} and get $\otil\left(K^{\frac{3}{4}}\right)$ regret, we only need to consider

% $\sum_{k=1}^K\sum_{h=1}^H\E_{s \sim \mu_h^k}\E_{a \sim \pi_k(\cdot|s)}\left[b_{k,h}(s,a)\right]$
\begin{align*}
&\E\left[\E_h^\star\left[\left\langle Q_{k,h}(s,\cdot) - B_{k,h}(s,a), \pi_k(\cdot|s) - \pi^\star(\cdot|s)\right\rangle\ind\{\calE_h\}\right] \right]
% \\&= \E_h^\star\left[\left\langle Q_{k,h}(s,\cdot) - B_{k,h}(s,a), \pi_k(\cdot|s) - \pi^\star(\cdot|s)\right\rangle\ind\{\calE_h\}\right] + \E_h^\star\left[\left\langle Q_{k,h}(s,\cdot) - B_{k,h}(s,a), \pi_k(\cdot|s) - \pi^\star(\cdot|s)\right\rangle\ind\{\calE_h\}\right]
\\&\le \underbrace{\E\left[\sum_{k=1}^K \sum_{h=1}^H \E_h^\star \left[ \left\langle Q_{k,h}(s, \cdot) - \widehat{Q}_{k,h}(s, \cdot), 
				\pi_k(\cdot|s) \right\rangle\ind\{\calE_h\}\right]
		\right]}_{\textbf{BIAS1}}
		+ \underbrace{\E\left[\sum_{k=1}^K \sum_{h=1}^H \E_h^\star\left[ \left\langle \widehat{Q}_{k,h}(s, \cdot) - Q_{k,h}(s, \cdot), 
				\pi^\star(\cdot|s) \right\rangle\ind\{\calE_h\}\right]
		\right]}_{\textbf{BIAS2}}
        \\
		&+ \underbrace{\E\left[\sum_{k=1}^K \sum_{h=1}^H \E_h^\star
			\left[ \left\langle \pmb{\widehat{\Gamma}}_{k,h} - \pmb{\widehat{B}}_{k,h}, 
				\pmb{H}_k(s) - \pmb{H}_{\star}(s) \right\rangle \ind\{\calE_h\}\right]
		\right]}_{\textbf{FTRL}} + \underbrace{\E\left[\sum_{k=1}^K \sum_{h=1}^H \E_h^\star \left[ \left\langle \widehat{B}_{k,h} - B_{k,h}, \pi_k(\cdot|s) - \pi^\star(\cdot|s) \right\rangle\ind\{\calE_h\} \right]\right]}_{\textbf{BIAS3}}
\end{align*}

To bound $\textbf{BIAS1}, \textbf{BIAS2}$, we utilize the matrix concentration bound derived in \cite{liu2023bypassing}, which is summarized in \pref{lem: matrix concentration} and is tailored for our setting.
\begin{lemma}[Lemma 19 in \cite{liu2023bypassing}] Define $\Sigma_{k,h} = \E_{s \sim \mu_h^k}\E_{a \sim \pi_k(\cdot|s)}\left[\phi(s,a)\phi(s,a)^\top\right]$ and $Q_{k,h}(s,a) = \phi(s,a)^\top{\rm q}_{k,h}$. If $\gamma = \order\left(\frac{d^3}{\tau}\right)$, then for any $k,h$,
\begin{equation*}
    \left\| \left(\hatSigma_{k,h} - \Sigma_{k,h} \right) {\rm q}_{k,h} \right\|_{\hatSigma^{-1}_{k,h}}^2 \le \order\left( \frac{d^{\frac{7}{2}}H}{\tau} \right)
\end{equation*}
\label{lem: matrix concentration}
\end{lemma}
With the help of this lemma, for any $s,a$, since $\tau = \order\left(K^{\frac{1}{2}}\right)$ and $\beta = \order\left(K^{-\frac{1}{4}}\right)$, we have
\begin{align*}
\E\left[Q_{k,h}(s,a) - \widehat{Q}_{k,h}(s,a)\right] &= \phi(s,a)^\top \left(\hatSigma_{k,h}\right)^{-1} \left(\hatSigma_{k,h} - \Sigma_{k,h} \right) {\rm q}_{k,h}  \le \|\phi(s,a)\|_{\hatSigma^{-1}_{k,h}} \left\|\left(\hatSigma_{k,h} - \Sigma_{k,h} \right) {\rm q}_{k,h} \right\|_{\hatSigma^{-1}_{k,h}}
\\&\le \sqrt{\frac{d^{\frac{7}{2}}H}{\tau}}\|\phi(s,a)\|_{\hatSigma^{-1}_{k,h}} \le \order\left(K^{-\frac{1}{4}}\right) + \beta\|\phi(s,a)\|_{\hatSigma^{-1}_{k,h}}^2
\end{align*}
where the expectation is for the randomness of $s_{k,h}, a_{k,h}$. The first inequality comes from Cauchy-Schwarz, the second inequality comes from \pref{lem: matrix concentration}, and the third inequality comes from AM-GM inequality. Thus, we have
\begin{align*}
    &\E\left[\textbf{BIAS1}\right] \le  \order\left(K^{\frac{3}{4}}\right) + \beta\sum_{k=1}^K \sum_{h=1}^H \E_h^\star\E_{a \sim \pi_h^k(\cdot|s)} \left[\|\phi(s,a)\|_{\hatSigma^{-1}_{k,h}}^2 \ind\{\calE_h\}\right]
\\ & \E\left[\textbf{BIAS2}\right] \le \order\left(K^{\frac{3}{4}}\right) + \beta\sum_{k=1}^K \sum_{h=1}^H \E_h^\star\E_{a \sim \pi_h^\star(\cdot|s)} \left[\|\phi(s,a)\|_{\hatSigma^{-1}_{k,h}}^2 \ind\{\calE_h\}\right]
\end{align*}

On the other hand, \textbf{BIAS3} can be directly bounded by \pref{lem: B main bias}. We have
\begin{align*}
    \textbf{BIAS3} \le \otil\left(K^{\frac{1}{2}}\right) + \alpha\sum_{k=1}^K \sum_{h=1}^H \E_h^\star\E_{a \sim \pi_k(\cdot|s)} \left[\|\phi(s,a)\|_{\Lambda^{-1}_{k,h}}^2 \ind\{\calE_h\}\right] + \alpha\sum_{k=1}^K \sum_{h=1}^H \E_h^\star\E_{a \sim \pi^\star(\cdot|s)} \left[\|\phi(s,a)\|_{\Lambda^{-1}_{k,h}}^2 \ind\{\calE_h\}\right]
\end{align*}

For the \textbf{FTRL} term, we analyze it in the lifted space and show that with $\eta = \frac{1}{2H^2}\beta = \order\left(K^{-\frac{1}{4}}\right)$ and $\alpha = \order\left(K^{\frac{3}{4}}\right)$, it has the following bound
\begin{align*}
    \textbf{FTRL} \le \otil\left(K^{\frac{3}{4}}\right) +\beta \sum_{k=1}^K\sum_{h=1}^H\E_h^\star\E_{a \sim \pi_k(\cdot|s)}\left[\|\phi(s,a)\|_{\hatSigma^{-1}_{k,h}}^2\ind\{\calE_h\}\right] +  \frac{1}{H}\sum_{k=1}^K\sum_{h=1}^H\E_h^\star\E_{a \sim \pi_k(\cdot|s)}\left[B_h^k(s,a)\ind\{\calE_h\}\right] 
\end{align*}
Thus, by combining all these terms, we could show
\begin{align*}
    &\E_h^\star\left[\left\langle Q_{k,h}(s,\cdot) - B_{k,h}(s,a), \pi_k(\cdot|s) - \pi^\star(\cdot|s)\right\rangle\ind\{\calE_h\}\right] 
    \\&\le \otil\left(K^{\frac{3}{4}}\right) +  \frac{1}{H}\sum_{k=1}^K\sum_{h=1}^H\E_h^\star\E_{a \sim \pi_k(\cdot|s)}\left[B_h^k(s,a)\ind\{\calE_h\}\right] 
    \\&\quad + \sum_{k=1}^K \sum_{h=1}^H \E_h^\star\E_{a \sim \pi^\star(\cdot|s)} \left[\left(\beta \|\phi(s,a)\|_{\hatSigma^{-1}_{k,h}}^2 + \alpha\|\phi(s,a)\|_{\Lambda^{-1}_{k,h}}^2\right)\ind\{\calE_h\}\right] 
   \\& \qquad +\sum_{k=1}^K \sum_{h=2}^H \E_h^\star\E_{a \sim \pi^\star(\cdot|s)} \left[\left(\E_{a \sim \pi_k(\cdot|s)}\left[\beta\|\phi(s,a)\|_{\hatSigma^{-1}_{k,h}}^2 + \alpha\|\phi(s,a)\|_{\Lambda^{-1}_{k,h}}^2\right]\right)\ind\{\calE_h\} \right] 
   \\&=  \otil\left(K^{\frac{3}{4}}\right) +  \sum_{k=1}^K\sum_{h=1}^H\E_h^\star\E_{a \sim \pi^\star(\cdot|s)}\left[b_{k,h}(s,a)\ind\{\calE_h\}\right] +  \frac{1}{H}\sum_{k=1}^K\sum_{h=1}^H\E_h^\star\E_{a \sim \pi_k(\cdot|s)}\left[B_h^k(s,a)\ind\{\calE_h\}\right] 
\end{align*}
Note that after the first inequality, we only take summation from $h=2$ to $h=H$. This is because $s_1$ is a fixed state and $\sum_{k=1}^K\E_{a \sim \pi_k(\cdot|s_1)}\left[\left(\beta\|\phi(s_1,a)\|_{\hatSigma^{-1}_{k,h}}^2 + \alpha\|\phi(s_1,a)\|_{\Lambda^{-1}_{k,h}}^2\right)\ind\{s_1 \in \calZ_1\}\right] \le \order\left(K^\frac{3}{4}\right)$. This part is absorbed in the first term. Thus, we could apply \pref{lem:dilated bonus bound} with $f(K) = \otil\left(K^{-\frac{1}{2}}\right)$ and $g(K) = \order\left(K^{\frac{3}{4}}\right)$. This leads to our regret bound of \pref{alg: logdet FTRL}
summarized in \pref{thm:eff reg}.
\begin{theorem}
\label{thm:eff reg}
\end{theorem}
